# Supplementary material for: Homotopy continuation method for solving Dyson equation fully self-consistently: theory and application to NdNiO2
Source: arXiv:2507.00290 source file (2025-06-30)
Supplement: Supplementary file 1 [file SI.pdf]

# Homotopy continuation method for solving Dyson equation self-consistently

Pavel Pokhilko[1,2,*] and Dominika Zgid[1,3]

[1]*Department of Chemistry, University of Michigan, Ann Arbor, Michigan 48109, USA*
[2]*Current address: Department of Physics and Astronomy, Purdue University, West Lafayette, Indiana 47907, USA*
[3]*Department of Physics, University of Michigan, Ann Arbor, Michigan 48109, USA*

## 1. GEOMETRY

```
Atomic positions in A:
Nd 1.96 1.96 1.64
Ni 0.0 0.0 0.0
O  0.0 1.96 0.0
O  1.96 0.0 0.0

Lattice vectors:
3.92 0.0 0.0
0.0 3.92 0.0
0.0 0.0 3.28
```

## 2. SOLUTIONS

### 2.1. NdNiO2

*Electronic address: pokhilko@umich.edu

TABLE S1: k-point occupations of UHF solutions 1 to 18.

| k-point coordinates | **1** | | **2** | | **3** | | **4** | | **5** | | **6** | |
|---|---|---|---|---|---|---|---|---|---|---|---|---|
| | $n_{k\alpha}$ | $n_{k\beta}$ | $n_{k\alpha}$ | $n_{k\beta}$ | $n_{k\alpha}$ | $n_{k\beta}$ | $n_{k\alpha}$ | $n_{k\beta}$ | $n_{k\alpha}$ | $n_{k\beta}$ | $n_{k\alpha}$ | $n_{k\beta}$ |
| (0, 0, 0) | 23.00 | 21.00 | 23.00 | 22.00 | 24.00 | 20.00 | 25.00 | 20.00 | 23.00 | 22.00 | 23.00 | 22.00 |
| (0, 0, 0.506847) | 23.00 | 21.00 | 23.00 | 21.00 | 24.00 | 20.00 | 24.00 | 20.00 | 23.00 | 21.00 | 23.00 | 21.00 |
| (0, 0.424097, 0) | 23.00 | 21.00 | 23.00 | 21.00 | 24.00 | 20.00 | 24.00 | 20.00 | 23.00 | 21.00 | 23.00 | 21.00 |
| (0, 0.424097, 0.506847) | 23.00 | 21.00 | 23.00 | 21.00 | 24.00 | 20.00 | 24.00 | 20.00 | 23.00 | 21.00 | 23.00 | 20.00 |
| (0.424097, 0, 0) | 23.00 | 21.00 | 23.00 | 21.00 | 24.00 | 20.00 | 24.00 | 20.00 | 23.00 | 21.00 | 23.00 | 22.00 |
| (0.424097, 0, 0.506847) | 23.00 | 21.00 | 23.00 | 20.00 | 24.00 | 20.00 | 24.00 | 20.00 | 23.00 | 20.00 | 23.00 | 20.00 |
| (0.424097, 0.424097, 0) | 23.00 | 21.00 | 23.00 | 21.00 | 24.00 | 20.00 | 23.00 | 20.00 | 23.00 | 21.00 | 23.00 | 21.00 |
| (0.424097, 0.424097, 0.506847) | 23.00 | 21.00 | 23.00 | 21.00 | 24.00 | 20.00 | 24.00 | 20.00 | 23.00 | 21.00 | 23.00 | 21.00 |

| k-point coordinates | **7** | | **8** | | **9** | | **10** | | **11** | | **13** | |
|---|---|---|---|---|---|---|---|---|---|---|---|---|
| | $n_{k\alpha}$ | $n_{k\beta}$ | $n_{k\alpha}$ | $n_{k\beta}$ | $n_{k\alpha}$ | $n_{k\beta}$ | $n_{k\alpha}$ | $n_{k\beta}$ | $n_{k\alpha}$ | $n_{k\beta}$ | $n_{k\alpha}$ | $n_{k\beta}$ |
| (0, 0, 0) | 23.00 | 22.00 | 23.00 | 22.00 | 23.00 | 22.00 | 23.00 | 22.00 | 23.00 | 22.00 | 24.00 | 22.00 |
| (0, 0, 0.506847) | 23.00 | 21.00 | 23.00 | 21.00 | 23.00 | 21.00 | 23.00 | 21.00 | 23.00 | 21.00 | 23.00 | 21.00 |
| (0, 0.424097, 0) | 23.00 | 21.00 | 23.00 | 21.00 | 23.00 | 21.00 | 23.00 | 21.00 | 23.00 | 22.00 | 23.00 | 21.00 |
| (0, 0.424097, 0.506847) | 23.00 | 20.00 | 23.00 | 21.00 | 23.00 | 21.00 | 23.00 | 21.00 | 23.00 | 20.00 | 23.00 | 20.00 |
| (0.424097, 0, 0) | 23.00 | 21.00 | 23.00 | 21.00 | 23.00 | 21.00 | 23.00 | 21.00 | 23.00 | 22.00 | 23.00 | 21.00 |
| (0.424097, 0, 0.506847) | 23.00 | 20.00 | 23.00 | 20.00 | 23.00 | 20.00 | 23.00 | 21.00 | 23.00 | 20.00 | 23.00 | 20.00 |
| (0.424097, 0.424097, 0) | 23.00 | 21.00 | 23.00 | 21.00 | 23.00 | 21.00 | 23.00 | 20.00 | 23.00 | 20.00 | 23.00 | 20.00 |
| (0.424097, 0.424097, 0.506847) | 24.00 | 21.00 | 23.00 | 21.00 | 23.00 | 21.00 | 23.00 | 21.00 | 23.00 | 21.00 | 24.00 | 21.00 |

| k-point coordinates | **14** | | **15** | | **16** | | **17** | | **18** | | | |
|---|---|---|---|---|---|---|---|---|---|---|---|---|
| | $n_{k\alpha}$ | $n_{k\beta}$ | $n_{k\alpha}$ | $n_{k\beta}$ | $n_{k\alpha}$ | $n_{k\beta}$ | $n_{k\alpha}$ | $n_{k\beta}$ | $n_{k\alpha}$ | $n_{k\beta}$ | $n_{k\alpha}$ | $n_{k\beta}$ |
| (0, 0, 0) | 24.00 | 22.00 | 24.00 | 22.00 | 24.00 | 22.00 | 24.00 | 21.00 | 23.00 | 22.00 | | |
| (0, 0, 0.506847) | 23.00 | 21.00 | 23.00 | 21.00 | 23.00 | 20.00 | 23.00 | 21.00 | 23.00 | 21.00 | | |
| (0, 0.424097, 0) | 23.00 | 21.00 | 23.00 | 21.00 | 23.00 | 22.00 | 24.00 | 21.00 | 23.00 | 22.00 | | |
| (0, 0.424097, 0.506847) | 23.00 | 20.00 | 23.00 | 20.00 | 23.00 | 20.00 | 23.00 | 20.00 | 23.00 | 20.00 | | |
| (0.424097, 0, 0) | 23.00 | 21.00 | 23.00 | 21.00 | 23.00 | 21.00 | 23.00 | 21.00 | 23.00 | 21.00 | | |
| (0.424097, 0, 0.506847) | 23.00 | 20.00 | 23.00 | 20.00 | 23.00 | 20.00 | 23.00 | 20.00 | 23.00 | 20.00 | | |
| (0.424097, 0.424097, 0) | 23.00 | 20.00 | 23.00 | 20.00 | 23.00 | 20.00 | 23.00 | 20.00 | 23.00 | 20.00 | | |
| (0.424097, 0.424097, 0.506847) | 24.00 | 21.00 | 24.00 | 21.00 | 24.00 | 21.00 | 24.00 | 21.00 | 24.00 | 21.00 | | |

TABLE S2: Lowdin k-resolved spin-summed orbital populations on Nd of the UHF **Solutions 1–8**.

| | **1** | | | | | **2** | | | | |
|---|---|---|---|---|---|---|---|---|---|---|
| k-point coordinates | $5d_{xy}$ | $5d_{yz}$ | $5d_{z^2}$ | $5d_{xz}$ | $5d_{x^2-y^2}$ | $5d_{xy}$ | $5d_{yz}$ | $5d_{z^2}$ | $5d_{xz}$ | $5d_{x^2-y^2}$ |
| (0, 0, 0) | 0.020 | 0.011 | 0.791 | 0.011 | 0.082 | 0.023 | 0.013 | 0.808 | 0.012 | 0.138 |
| (0, 0, 0.506847) | 0.000 | 0.320 | 0.560 | 0.320 | 0.327 | 0.000 | 0.326 | 0.575 | 0.326 | 0.336 |
| (0, 0.424097, 0) | 0.135 | 0.205 | 0.908 | 0.000 | 0.127 | 0.137 | 0.209 | 0.914 | 0.000 | 0.129 |
| (0, 0.424097, 0.506847) | 0.941 | 0.163 | 0.051 | 0.319 | 0.181 | 0.942 | 0.165 | 0.051 | 0.325 | 0.186 |
| (0.424097, 0, 0) | 0.135 | 0.000 | 0.908 | 0.205 | 0.127 | 0.131 | 0.000 | 0.913 | 0.209 | 0.129 |
| (0.424097, 0, 0.506847) | **0.941** | 0.319 | 0.051 | 0.163 | 0.181 | **0.045** | 0.325 | 0.052 | 0.165 | 0.186 |
| (0.424097, 0.424097, 0) | 0.247 | 0.196 | 1.031 | 0.196 | 0.138 | 0.253 | 0.200 | 1.033 | 0.199 | 0.143 |
| (0.424097, 0.424097, 0.506847) | 0.617 | 0.119 | 0.011 | 0.119 | 0.000 | 0.602 | 0.120 | 0.011 | 0.120 | 0.000 |

| | **3** | | | | | **4** | | | | |
|---|---|---|---|---|---|---|---|---|---|---|
| k-point coordinates | $5d_{xy}$ | $5d_{yz}$ | $5d_{z^2}$ | $5d_{xz}$ | $5d_{x^2-y^2}$ | $5d_{xy}$ | $5d_{yz}$ | $5d_{z^2}$ | $5d_{xz}$ | $5d_{x^2-y^2}$ |
| (0, 0, 0) | 0.061 | 0.029 | **0.113** | 0.029 | 0.092 | 0.056 | 0.027 | **0.890** | 0.027 | 0.092 |
| (0, 0, 0.506847) | 0.000 | 0.371 | 0.122 | 0.371 | 0.375 | 0.000 | 0.360 | 0.122 | 0.360 | 0.364 |
| (0, 0.424097, 0) | 0.148 | 0.239 | 0.114 | 0.000 | 0.127 | 0.151 | 0.230 | 0.121 | 0.000 | 0.124 |
| (0, 0.424097, 0.506847) | 0.110 | 0.197 | 0.053 | 0.369 | 0.215 | 0.102 | 0.195 | 0.052 | 0.357 | 0.208 |
| (0.424097, 0, 0) | 0.148 | 0.000 | 0.114 | 0.239 | 0.127 | 0.151 | 0.000 | 0.121 | 0.230 | 0.124 |
| (0.424097, 0, 0.506847) | 0.110 | 0.369 | 0.053 | 0.197 | 0.215 | 0.102 | 0.357 | 0.053 | 0.195 | 0.208 |
| (0.424097, 0.424097, 0) | 0.339 | 0.229 | 0.187 | 0.229 | 0.167 | 0.329 | 0.220 | 0.186 | 0.220 | 0.161 |
| (0.424097, 0.424097, 0.506847) | 0.682 | 0.128 | 0.010 | 0.128 | 0.000 | 0.675 | 0.126 | 0.010 | 0.126 | 0.000 |

| | **5** | | | | | **6** | | | | |
|---|---|---|---|---|---|---|---|---|---|---|
| k-point coordinates | $5d_{xy}$ | $5d_{yz}$ | $5d_{z^2}$ | $5d_{xz}$ | $5d_{x^2-y^2}$ | $5d_{xy}$ | $5d_{yz}$ | $5d_{z^2}$ | $5d_{xz}$ | $5d_{x^2-y^2}$ |
| (0, 0, 0) | 0.034 | 0.016 | 0.854 | 0.016 | 0.096 | 0.031 | 0.014 | 0.881 | 0.014 | 0.092 |
| (0, 0, 0.506847) | 0.000 | 0.335 | 0.131 | 0.335 | 0.354 | 0.000 | 0.335 | 0.132 | 0.332 | 0.353 |
| (0, 0.424097, 0) | 0.139 | 0.217 | 0.922 | 0.000 | 0.131 | 0.134 | 0.218 | 0.921 | 0.000 | 0.130 |
| (0, 0.424097, 0.506847) | 0.060 | 0.171 | 0.055 | 0.333 | 0.199 | 0.052 | 0.171 | 0.055 | 0.330 | 0.196 |
| (0.424097, 0, 0) | 0.138 | 0.000 | 0.924 | 0.218 | 0.130 | 0.140 | 0.000 | 0.925 | 0.216 | 0.128 |
| (0.424097, 0, 0.506847) | 0.058 | 0.333 | 0.055 | 0.167 | 0.199 | 0.052 | 0.333 | 0.055 | 0.166 | 0.198 |
| (0.424097, 0.424097, 0) | 0.269 | 0.208 | 1.035 | 0.208 | 0.151 | 0.268 | 0.208 | 1.032 | 0.206 | 0.150 |
| (0.424097, 0.424097, 0.506847) | 0.595 | 0.122 | 0.012 | 0.122 | 0.000 | 0.578 | 0.122 | 0.012 | 0.121 | 0.000 |

| | **7** | | | | | **8** | | | | |
|---|---|---|---|---|---|---|---|---|---|---|
| k-point coordinates | $5d_{xy}$ | $5d_{yz}$ | $5d_{z^2}$ | $5d_{xz}$ | $5d_{x^2-y^2}$ | $5d_{xy}$ | $5d_{yz}$ | $5d_{z^2}$ | $5d_{xz}$ | $5d_{x^2-y^2}$ |
| (0, 0, 0) | 0.027 | 0.015 | 0.844 | 0.015 | 0.099 | 0.028 | 0.015 | 0.832 | 0.014 | 0.098 |
| (0, 0, 0.506847) | 0.000 | 0.329 | 0.128 | 0.329 | 0.344 | 0.000 | 0.327 | 0.127 | 0.327 | 0.341 |
| (0, 0.424097, 0) | 0.135 | 0.213 | 0.925 | 0.000 | 0.127 | 0.140 | 0.211 | 0.919 | 0.000 | 0.128 |
| (0, 0.424097, 0.506847) | **0.055** | 0.167 | 0.053 | 0.326 | 0.192 | **0.951** | 0.166 | 0.053 | 0.324 | 0.191 |
| (0.424097, 0, 0) | 0.135 | 0.000 | 0.925 | 0.213 | 0.127 | 0.135 | 0.000 | 0.918 | 0.211 | 0.127 |
| (0.424097, 0, 0.506847) | 0.055 | 0.326 | 0.053 | 0.167 | 0.192 | 0.053 | 0.325 | 0.054 | 0.166 | 0.190 |
| (0.424097, 0.424097, 0) | 0.270 | 0.203 | 1.030 | 0.203 | 0.145 | 0.265 | 0.202 | 1.031 | 0.202 | 0.144 |
| (0.424097, 0.424097, 0.506847) | **1.221** | 0.120 | 0.011 | 0.120 | 0.000 | **0.618** | 0.120 | 0.011 | 0.120 | 0.000 |

TABLE S3: Lowdin k-resolved spin-summed orbital populations on Nd of the UHF **Solutions 9–11, 13–17**.

| | **9** | | | | | **10** | | | | |
|---|---|---|---|---|---|---|---|---|---|---|
| k-point coordinates | $5d_{xy}$ | $5d_{yz}$ | $5d_{z^2}$ | $5d_{xz}$ | $5d_{x^2-y^2}$ | $5d_{xy}$ | $5d_{yz}$ | $5d_{z^2}$ | $5d_{xz}$ | $5d_{x^2-y^2}$ |
| (0, 0, 0) | 0.032 | 0.017 | 0.851 | 0.017 | 0.093 | 0.056 | 0.027 | 0.860 | 0.027 | 0.091 |
| (0, 0, 0.506847) | 0.000 | 0.331 | 0.128 | 0.334 | 0.350 | 0.000 | 0.360 | 0.122 | 0.360 | 0.364 |
| (0, 0.424097, 0) | 0.139 | 0.214 | 0.925 | 0.000 | 0.129 | 0.148 | 0.230 | 0.117 | 0.000 | 0.124 |
| (0, 0.424097, 0.506847) | 0.061 | 0.180 | 0.055 | 0.332 | 0.197 | 0.102 | 0.194 | 0.052 | 0.357 | 0.208 |
| (0.424097, 0, 0) | 0.136 | 0.000 | 0.925 | 0.216 | 0.129 | 0.148 | 0.000 | 0.117 | 0.230 | 0.124 |
| (0.424097, 0, 0.506847) | 0.062 | 0.328 | 0.054 | 0.168 | 0.195 | 0.102 | 0.357 | 0.052 | 0.194 | 0.208 |
| (0.424097, 0.424097, 0) | 0.274 | 0.204 | 1.034 | 0.207 | 0.149 | 0.329 | 0.220 | 0.184 | 0.220 | 0.160 |
| (0.424097, 0.424097, 0.506847) | 0.603 | 0.121 | 0.011 | 0.122 | 0.000 | 0.639 | 0.126 | 0.010 | 0.126 | 0.000 |

| | **11** | | | | | **13** | | | | |
|---|---|---|---|---|---|---|---|---|---|---|
| k-point coordinates | $5d_{xy}$ | $5d_{yz}$ | $5d_{z^2}$ | $5d_{xz}$ | $5d_{x^2-y^2}$ | $5d_{xy}$ | $5d_{yz}$ | $5d_{z^2}$ | $5d_{xz}$ | $5d_{x^2-y^2}$ |
| (0, 0, 0) | 0.040 | 0.020 | 0.840 | 0.020 | 0.091 | 0.028 | 0.015 | 1.541 | 0.015 | 0.099 |
| (0, 0, 0.506847) | 0.000 | 0.342 | 0.126 | 0.342 | 0.353 | 0.000 | 0.332 | 0.130 | 0.332 | 0.344 |
| (0, 0.424097, 0) | 0.142 | 0.219 | 0.902 | 0.000 | 0.140 | 0.134 | 0.214 | 0.897 | 0.000 | 0.142 |
| (0, 0.424097, 0.506847) | 0.074 | 0.171 | 0.054 | 0.339 | 0.199 | 0.056 | 0.168 | 0.053 | 0.330 | 0.193 |
| (0.424097, 0, 0) | 0.142 | 0.000 | 0.902 | 0.219 | 0.140 | 0.134 | 0.000 | 0.897 | 0.214 | 0.142 |
| (0.424097, 0, 0.506847) | 0.074 | 0.339 | 0.054 | 0.171 | 0.199 | 0.056 | 0.330 | 0.053 | 0.168 | 0.193 |
| (0.424097, 0.424097, 0) | 0.294 | 0.210 | 0.176 | 0.210 | 0.151 | 0.270 | 0.205 | 0.166 | 0.205 | 0.145 |
| (0.424097, 0.424097, 0.506847) | 0.617 | 0.123 | 0.011 | 0.123 | 0.000 | 1.229 | 0.121 | 0.011 | 0.121 | 0.000 |

| | **14** | | | | | **15** | | | | |
|---|---|---|---|---|---|---|---|---|---|---|
| k-point coordinates | $5d_{xy}$ | $5d_{yz}$ | $5d_{z^2}$ | $5d_{xz}$ | $5d_{x^2-y^2}$ | $5d_{xy}$ | $5d_{yz}$ | $5d_{z^2}$ | $5d_{xz}$ | $5d_{x^2-y^2}$ |
| (0, 0, 0) | 0.028 | 0.015 | 0.821 | 0.015 | 0.967 | 0.033 | 0.015 | 1.564 | 0.015 | 0.106 |
| (0, 0, 0.506847) | 0.000 | 0.333 | 0.125 | 0.333 | 0.355 | 0.000 | 0.341 | 0.132 | 0.342 | 0.353 |
| (0, 0.424097, 0) | 0.133 | 0.215 | 0.902 | 0.000 | 0.138 | 0.140 | 0.220 | 0.119 | 0.000 | 0.119 |
| (0, 0.424097, 0.506847) | 0.055 | 0.168 | 0.052 | 0.331 | 0.197 | 0.056 | 0.168 | 0.052 | 0.341 | 0.198 |
| (0.424097, 0, 0) | 0.133 | 6.145 | 0.902 | 0.215 | 0.138 | 0.136 | 0.000 | 0.875 | 0.222 | 0.158 |
| (0.424097, 0, 0.506847) | 0.055 | 0.331 | 0.052 | 0.168 | 0.197 | 0.056 | 0.339 | 0.054 | 0.173 | 0.197 |
| (0.424097, 0.424097, 0) | 0.267 | 0.205 | 0.163 | 0.205 | 0.147 | 0.278 | 0.210 | 0.171 | 0.212 | 0.150 |
| (0.424097, 0.424097, 0.506847) | 1.222 | 0.121 | 0.011 | 0.121 | 0.000 | 1.219 | 0.122 | 0.011 | 0.123 | 0.000 |

| | **16** | | | | | **17** | | | | |
|---|---|---|---|---|---|---|---|---|---|---|
| k-point coordinates | $5d_{xy}$ | $5d_{yz}$ | $5d_{z^2}$ | $5d_{xz}$ | $5d_{x^2-y^2}$ | $5d_{xy}$ | $5d_{yz}$ | $5d_{z^2}$ | $5d_{xz}$ | $5d_{x^2-y^2}$ |
| (0, 0, 0) | 0.030 | 0.014 | 1.483 | 0.052 | 0.116 | 0.030 | 0.014 | 1.246 | 0.014 | 0.090 |
| (0, 0, 0.506847) | 0.000 | 0.335 | 0.135 | 0.338 | 0.352 | 0.000 | 0.338 | 0.135 | 0.339 | 0.352 |
| (0, 0.424097, 0) | 0.135 | 0.218 | 0.891 | 0.000 | 0.145 | 0.138 | 0.220 | 0.865 | 0.000 | 0.170 |
| (0, 0.424097, 0.506847) | 0.042 | 0.169 | 0.055 | 0.336 | 0.197 | 0.051 | 0.168 | 0.055 | 0.338 | 0.197 |
| (0.424097, 0, 0) | 0.135 | 0.000 | 0.888 | 0.220 | 0.147 | 0.135 | 0.000 | 0.820 | 0.221 | 0.186 |
| (0.424097, 0, 0.506847) | 0.052 | 0.333 | 0.056 | 0.170 | 0.191 | 0.051 | 0.336 | 0.054 | 0.171 | 0.196 |
| (0.424097, 0.424097, 0) | 0.264 | 0.209 | 0.168 | 0.209 | 0.147 | 0.271 | 0.210 | 0.168 | 0.210 | 0.147 |
| (0.424097, 0.424097, 0.506847) | 1.208 | 0.121 | 0.011 | 0.122 | 0.000 | 1.205 | 0.122 | 0.011 | 0.122 | 0.000 |

TABLE S4: Lowdin k-resolved spin-summed orbital populations on Nd of the UHF **Solutions 18**.

| | **18** | | | | | | | | | |
|---|---|---|---|---|---|---|---|---|---|---|
| k-point coordinates | $5d_{xy}$ | $5d_{yz}$ | $5d_{z^2}$ | $5d_{xz}$ | $5d_{x^2-y^2}$ | $5d_{xy}$ | $5d_{yz}$ | $5d_{z^2}$ | $5d_{xz}$ | $5d_{x^2-y^2}$ |
| (0, 0, 0) | 0.032 | 0.015 | 0.874 | 0.015 | 0.093 | | | | | |
| (0, 0, 0.506847) | 0.000 | 0.338 | 0.130 | 0.340 | 0.352 | | | | | |
| (0, 0.424097, 0) | 0.141 | 0.219 | 0.905 | 0.000 | 0.136 | | | | | |
| (0, 0.424097, 0.506847) | 0.055 | 0.168 | 0.054 | 0.338 | 0.197 | | | | | |
| (0.424097, 0, 0) | 0.136 | 0.000 | 0.899 | 0.221 | 0.138 | | | | | |
| (0.424097, 0, 0.506847) | 0.055 | 0.337 | 0.054 | 0.172 | 0.196 | | | | | |
| (0.424097, 0.424097, 0) | 0.277 | 0.209 | 0.171 | 0.211 | 0.149 | | | | | |
| (0.424097, 0.424097, 0.506847) | 1.216 | 0.122 | 0.011 | 0.122 | 0.000 | | | | | |

TABLE S5: Lowdin k-resolved spin-summed orbital populations on Ni of UHF **Solutions 1–8**.

| | **1** | | | | | **2** | | | | |
|---|---|---|---|---|---|---|---|---|---|---|
| k-point coordinates | $5d_{xy}$ | $5d_{yz}$ | $5d_{z^2}$ | $5d_{xz}$ | $5d_{x^2-y^2}$ | $5d_{xy}$ | $5d_{yz}$ | $5d_{z^2}$ | $5d_{xz}$ | $5d_{x^2-y^2}$ |
| (0, 0, 0) | 1.619 | 1.680 | 1.653 | 1.680 | 0.054 | 1.625 | 1.689 | 1.651 | 1.687 | 0.853 |
| (0, 0, 0.506847) | 1.631 | 1.661 | 1.666 | 1.661 | 0.058 | 1.639 | 1.667 | 1.672 | 1.666 | 0.058 |
| (0, 0.424097, 0) | 1.624 | 1.652 | 1.649 | 1.678 | 0.191 | 1.632 | 1.661 | 1.649 | 1.685 | 0.205 |
| (0, 0.424097, 0.506847) | 1.606 | 1.651 | 1.658 | 1.616 | 0.209 | 1.614 | 1.658 | 1.664 | 1.619 | 0.219 |
| (0.424097, 0, 0) | 1.624 | 1.678 | 1.649 | 1.652 | 0.191 | 1.632 | 1.686 | 1.650 | 1.659 | 0.205 |
| (0.424097, 0, 0.506847) | 1.606 | 1.616 | 1.658 | 1.651 | 0.209 | 1.614 | 1.611 | 1.664 | 1.657 | 0.220 |
| (0.424097, 0.424097, 0) | 1.609 | 1.642 | 1.589 | 1.642 | 0.412 | 1.617 | 1.650 | 1.585 | 1.649 | 0.429 |
| (0.424097, 0.424097, 0.506847) | 1.607 | 1.657 | 1.649 | 1.657 | 0.417 | 1.615 | 1.665 | 1.655 | 1.664 | 0.429 |

| | **3** | | | | | **4** | | | | |
|---|---|---|---|---|---|---|---|---|---|---|
| k-point coordinates | $5d_{xy}$ | $5d_{yz}$ | $5d_{z^2}$ | $5d_{xz}$ | $5d_{x^2-y^2}$ | $5d_{xy}$ | $5d_{yz}$ | $5d_{z^2}$ | $5d_{xz}$ | $5d_{x^2-y^2}$ |
| (0, 0, 0) | 1.651 | 1.723 | 1.461 | 1.723 | 0.825 | 1.651 | 1.722 | 1.558 | 1.722 | 0.833 |
| (0, 0, 0.506847) | 1.682 | 1.689 | 1.707 | 1.689 | 0.829 | 1.679 | 1.689 | 1.704 | 1.689 | 0.837 |
| (0, 0.424097, 0) | 1.681 | 1.699 | 1.615 | 1.724 | 0.842 | 1.677 | 1.696 | 1.625 | 1.722 | 0.846 |
| (0, 0.424097, 0.506847) | 1.662 | 1.687 | 1.696 | 1.589 | 0.844 | 1.658 | 1.685 | 1.693 | 1.594 | 0.849 |
| (0.424097, 0, 0) | 1.681 | 1.724 | 1.615 | 1.699 | 0.842 | 1.677 | 1.722 | 1.625 | 1.696 | 0.846 |
| (0.424097, 0, 0.506847) | 1.662 | 1.589 | 1.696 | 1.687 | 0.844 | 1.658 | 1.594 | 1.693 | 1.685 | 0.849 |
| (0.424097, 0.424097, 0) | 1.663 | 1.688 | 1.503 | 1.688 | 0.873 | 1.659 | 1.686 | 1.519 | 1.686 | 0.635 |
| (0.424097, 0.424097, 0.506847) | 1.665 | 1.698 | 1.688 | 1.698 | 0.652 | 1.661 | 1.697 | 1.685 | 1.697 | 0.640 |

| | **5** | | | | | **6** | | | | |
|---|---|---|---|---|---|---|---|---|---|---|
| k-point coordinates | $5d_{xy}$ | $5d_{yz}$ | $5d_{z^2}$ | $5d_{xz}$ | $5d_{x^2-y^2}$ | $5d_{xy}$ | $5d_{yz}$ | $5d_{z^2}$ | $5d_{xz}$ | $5d_{x^2-y^2}$ |
| (0, 0, 0) | 1.642 | 1.703 | 1.525 | 1.704 | 0.915 | 1.640 | 1.697 | 1.394 | 1.697 | 0.826 |
| (0, 0, 0.506847) | 1.660 | 1.678 | 1.576 | 1.679 | 0.967 | 1.656 | 1.674 | 1.543 | 1.673 | 0.974 |
| (0, 0.424097, 0) | 1.655 | 1.675 | 1.369 | 1.702 | 0.431 | 1.651 | 1.669 | 1.255 | 1.694 | 0.526 |
| (0, 0.424097, 0.506847) | 1.637 | 1.671 | 1.588 | 1.612 | 0.983 | 1.633 | 1.666 | 1.209 | 1.612 | 0.566 |
| (0.424097, 0, 0) | 1.655 | 1.701 | 1.391 | 1.676 | 0.464 | 1.651 | 1.695 | 1.433 | 1.668 | 0.861 |
| (0.424097, 0, 0.506847) | 1.637 | 1.612 | 1.366 | 1.672 | 0.517 | 1.633 | 1.612 | 1.220 | 1.666 | 0.582 |
| (0.424097, 0.424097, 0) | 1.639 | 1.664 | 1.408 | 1.666 | 0.587 | 1.636 | 1.659 | 1.319 | 1.658 | 0.631 |
| (0.424097, 0.424097, 0.506847) | 1.638 | 1.678 | 1.450 | 1.680 | 0.612 | 1.634 | 1.673 | 1.320 | 1.673 | 0.648 |

| | **7** | | | | | **8** | | | | |
|---|---|---|---|---|---|---|---|---|---|---|
| k-point coordinates | $5d_{xy}$ | $5d_{yz}$ | $5d_{z^2}$ | $5d_{xz}$ | $5d_{x^2-y^2}$ | $5d_{xy}$ | $5d_{yz}$ | $5d_{z^2}$ | $5d_{xz}$ | $5d_{x^2-y^2}$ |
| (0, 0, 0) | 1.633 | 1.697 | 1.638 | 1.697 | 0.868 | 1.633 | 1.698 | 1.644 | 1.696 | 0.868 |
| (0, 0, 0.506847) | 1.648 | 1.673 | 1.679 | 1.673 | 0.876 | 1.648 | 1.674 | 1.680 | 1.673 | 0.876 |
| (0, 0.424097, 0) | 1.642 | 1.668 | 1.647 | 1.694 | 0.229 | 1.642 | 1.669 | 1.649 | 1.694 | 0.231 |
| (0, 0.424097, 0.506847) | 1.624 | 1.665 | 1.671 | 1.610 | 0.253 | 1.624 | 1.666 | 1.672 | 1.623 | 0.254 |
| (0.424097, 0, 0) | 1.642 | 1.694 | 1.647 | 1.668 | 0.229 | 1.642 | 1.695 | 1.650 | 1.668 | 0.231 |
| (0.424097, 0, 0.506847) | 1.624 | 1.610 | 1.671 | 1.665 | 0.253 | 1.624 | 1.612 | 1.672 | 1.665 | 0.256 |
| (0.424097, 0.424097, 0) | 1.627 | 1.658 | 1.575 | 1.658 | 0.455 | 1.627 | 1.659 | 1.579 | 1.658 | 0.458 |
| (0.424097, 0.424097, 0.506847) | 1.625 | 1.672 | 1.662 | 1.672 | 0.460 | 1.625 | 1.673 | 1.663 | 1.672 | 0.463 |

TABLE S6: Lowdin k-resolved spin-summed orbital populations on Ni of UHF **Solutions 9–11, 13–17**.

| | **9** | | | | | **10** | | | | |
|---|---|---|---|---|---|---|---|---|---|---|
| k-point coordinates | $5d_{xy}$ | $5d_{yz}$ | $5d_{z^2}$ | $5d_{xz}$ | $5d_{x^2-y^2}$ | $5d_{xy}$ | $5d_{yz}$ | $5d_{z^2}$ | $5d_{xz}$ | $5d_{x^2-y^2}$ |
| (0, 0, 0) | 1.640 | 1.705 | 1.629 | 1.704 | 0.860 | 1.651 | 1.721 | 1.549 | 1.721 | 0.833 |
| (0, 0, 0.506847) | 1.657 | 1.679 | 1.683 | 1.679 | 0.867 | 1.679 | 1.689 | 1.703 | 1.689 | 0.837 |
| (0, 0.424097, 0) | 1.651 | 1.677 | 1.641 | 1.702 | 0.255 | 1.677 | 1.696 | 1.622 | 1.722 | 0.847 |
| (0, 0.424097, 0.506847) | 1.633 | 1.672 | 1.674 | 1.611 | 0.875 | 1.658 | 1.685 | 1.693 | 1.593 | 0.850 |
| (0.424097, 0, 0) | 1.651 | 1.703 | 1.643 | 1.676 | 0.276 | 1.677 | 1.722 | 1.622 | 1.696 | 0.847 |
| (0.424097, 0, 0.506847) | 1.633 | 1.611 | 1.675 | 1.671 | 0.309 | 1.658 | 1.593 | 1.693 | 1.685 | 0.850 |
| (0.424097, 0.424097, 0) | 1.636 | 1.667 | 1.566 | 1.666 | 0.496 | 1.659 | 1.686 | 1.516 | 1.686 | 0.634 |
| (0.424097, 0.424097, 0.506847) | 1.634 | 1.680 | 1.665 | 1.679 | 0.510 | 1.661 | 1.696 | 1.685 | 1.696 | 0.638 |

| | **11** | | | | | **13** | | | | |
|---|---|---|---|---|---|---|---|---|---|---|
| k-point coordinates | $5d_{xy}$ | $5d_{yz}$ | $5d_{z^2}$ | $5d_{xz}$ | $5d_{x^2-y^2}$ | $5d_{xy}$ | $5d_{yz}$ | $5d_{z^2}$ | $5d_{xz}$ | $5d_{x^2-y^2}$ |
| (0, 0, 0) | 1.645 | 1.712 | 1.616 | 1.712 | 0.851 | 1.633 | 1.697 | 1.680 | 1.697 | 0.868 |
| (0, 0, 0.506847) | 1.666 | 1.683 | 1.694 | 1.683 | 0.856 | 1.649 | 1.674 | 1.679 | 1.674 | 0.876 |
| (0, 0.424097, 0) | 1.662 | 1.684 | 1.643 | 1.710 | 0.860 | 1.643 | 1.669 | 1.649 | 1.695 | 0.224 |
| (0, 0.424097, 0.506847) | 1.643 | 1.678 | 1.680 | 1.607 | 0.354 | 1.625 | 1.666 | 1.670 | 1.609 | 0.248 |
| (0.424097, 0, 0) | 1.662 | 1.710 | 1.643 | 1.684 | 0.860 | 1.643 | 1.695 | 1.649 | 1.669 | 0.224 |
| (0.424097, 0, 0.506847) | 1.643 | 1.607 | 1.680 | 1.678 | 0.354 | 1.625 | 1.609 | 1.670 | 1.666 | 0.248 |
| (0.424097, 0.424097, 0) | 1.645 | 1.674 | 1.555 | 1.674 | 0.557 | 1.627 | 1.659 | 1.576 | 1.659 | 0.447 |
| (0.424097, 0.424097, 0.506847) | 1.645 | 1.687 | 1.675 | 1.687 | 0.546 | 1.626 | 1.673 | 1.661 | 1.673 | 0.452 |

| | **14** | | | | | **15** | | | | |
|---|---|---|---|---|---|---|---|---|---|---|
| k-point coordinates | $5d_{xy}$ | $5d_{yz}$ | $5d_{z^2}$ | $5d_{xz}$ | $5d_{x^2-y^2}$ | $5d_{xy}$ | $5d_{yz}$ | $5d_{z^2}$ | $5d_{xz}$ | $5d_{x^2-y^2}$ |
| (0, 0, 0) | 1.633 | 1.696 | 1.638 | 1.696 | 0.887 | 1.640 | 1.697 | 1.387 | 1.697 | 0.861 |
| (0, 0, 0.506847) | 1.648 | 1.673 | 1.679 | 1.673 | 0.876 | 1.658 | 1.673 | 1.526 | 1.673 | 0.991 |
| (0, 0.424097, 0) | 1.642 | 1.668 | 1.648 | 1.694 | 0.228 | 1.652 | 1.669 | 1.412 | 1.694 | 0.869 |
| (0, 0.424097, 0.506847) | 1.624 | 1.665 | 1.671 | 1.610 | 0.251 | 1.634 | 1.665 | 1.194 | 1.609 | 0.596 |
| (0.424097, 0, 0) | 1.642 | 1.694 | 1.648 | 1.668 | 0.228 | 1.652 | 1.695 | 1.232 | 1.668 | 0.537 |
| (0.424097, 0, 0.506847) | 1.624 | 1.610 | 1.671 | 1.665 | 0.251 | 1.634 | 1.609 | 1.182 | 1.665 | 0.582 |
| (0.424097, 0.424097, 0) | 1.627 | 1.658 | 1.575 | 1.658 | 0.452 | 1.636 | 1.658 | 1.294 | 1.658 | 0.632 |
| (0.424097, 0.424097, 0.506847) | 1.625 | 1.672 | 1.662 | 1.672 | 0.457 | 1.635 | 1.673 | 1.291 | 1.672 | 0.653 |

| | **16** | | | | | **17** | | | | |
|---|---|---|---|---|---|---|---|---|---|---|
| k-point coordinates | $5d_{xy}$ | $5d_{yz}$ | $5d_{z^2}$ | $5d_{xz}$ | $5d_{x^2-y^2}$ | $5d_{xy}$ | $5d_{yz}$ | $5d_{z^2}$ | $5d_{xz}$ | $5d_{x^2-y^2}$ |
| (0, 0, 0) | 1.637 | 1.695 | 1.602 | 1.581 | 1.003 | 1.638 | 1.692 | 1.167 | 1.693 | 0.648 |
| (0, 0, 0.506847) | 1.654 | 1.672 | 1.555 | 1.280 | 0.517 | 1.654 | 1.670 | 1.504 | 1.670 | 1.006 |
| (0, 0.424097, 0) | 1.648 | 1.667 | 1.612 | 1.590 | 1.000 | 1.649 | 1.664 | 1.373 | 1.690 | 0.857 |
| (0, 0.424097, 0.506847) | 1.630 | 1.664 | 1.563 | 1.284 | 0.553 | 1.631 | 1.662 | 1.168 | 1.610 | 0.606 |
| (0.424097, 0, 0) | 1.648 | 1.692 | 1.560 | 1.298 | 0.579 | 1.649 | 1.690 | 1.199 | 1.665 | 0.555 |
| (0.424097, 0, 0.506847) | 1.630 | 1.611 | 1.561 | 1.308 | 0.580 | 1.631 | 1.610 | 1.153 | 1.662 | 0.597 |
| (0.424097, 0.424097, 0) | 1.632 | 1.656 | 1.520 | 1.373 | 0.651 | 1.633 | 1.654 | 1.264 | 1.654 | 0.641 |
| (0.424097, 0.424097, 0.506847) | 1.631 | 1.671 | 1.575 | 1.388 | 0.652 | 1.632 | 1.668 | 1.258 | 1.669 | 0.663 |

TABLE S7: Lowdin k-resolved spin-summed orbital populations on Ni of UHF **Solution 18**.

| | **18** | | | | | | | | | |
|---|---|---|---|---|---|---|---|---|---|---|
| k-point coordinates | $5d_{xy}$ | $5d_{yz}$ | $5d_{z^2}$ | $5d_{xz}$ | $5d_{x^2-y^2}$ | $5d_{xy}$ | $5d_{yz}$ | $5d_{z^2}$ | $5d_{xz}$ | $5d_{x^2-y^2}$ |
| (0, 0, 0) | 1.640 | 1.696 | 1.388 | 1.696 | 0.827 | | | | | |
| (0, 0, 0.506847) | 1.657 | 1.672 | 1.542 | 1.673 | 0.976 | | | | | |
| (0, 0.424097, 0) | 1.652 | 1.668 | 1.426 | 1.694 | 0.861 | | | | | |
| (0, 0.424097, 0.506847) | 1.633 | 1.665 | 1.206 | 1.610 | 0.590 | | | | | |
| (0.424097, 0, 0) | 1.652 | 1.694 | 1.241 | 1.668 | 0.531 | | | | | |
| (0.424097, 0, 0.506847) | 1.633 | 1.609 | 1.192 | 1.665 | 0.574 | | | | | |
| (0.424097, 0.424097, 0) | 1.635 | 1.657 | 1.304 | 1.658 | 0.630 | | | | | |
| (0.424097, 0.424097, 0.506847) | 1.634 | 1.672 | 1.304 | 1.672 | 0.650 | | | | | |

TABLE S8: Lowdin k-resolved spin-summed orbital populations on Nd of scGW **Solutions 3–7, 10–12**.

| | **3** | | | | | **4** | | | | |
|---|---|---|---|---|---|---|---|---|---|---|
| k-point coordinates | $5d_{xy}$ | $5d_{yz}$ | $5d_{z^2}$ | $5d_{xz}$ | $5d_{x^2-y^2}$ | $5d_{xy}$ | $5d_{yz}$ | $5d_{z^2}$ | $5d_{xz}$ | $5d_{x^2-y^2}$ |
| (0, 0, 0) | 0.126 | 0.062 | 0.319 | 0.062 | 0.118 | 0.117 | 0.059 | 0.955 | 0.059 | 0.117 |
| (0, 0, 0.506847) | 0.017 | 0.422 | 0.165 | 0.422 | 0.434 | 0.017 | 0.413 | 0.166 | 0.413 | 0.426 |
| (0, 0.424097, 0) | 0.196 | 0.280 | 0.178 | 0.017 | 0.152 | 0.193 | 0.272 | 0.182 | 0.017 | 0.150 |
| (0, 0.424097, 0.506847) | 0.214 | 0.239 | 0.077 | 0.425 | 0.259 | 0.202 | 0.235 | 0.077 | 0.415 | 0.253 |
| (0.424097, 0, 0) | 0.196 | 0.017 | 0.178 | 0.280 | 0.152 | 0.193 | 0.017 | 0.182 | 0.272 | 0.150 |
| (0.424097, 0, 0.506847) | 0.214 | 0.425 | 0.077 | 0.239 | 0.259 | 0.202 | 0.415 | 0.077 | 0.235 | 0.253 |
| (0.424097, 0.424097, 0) | 0.433 | 0.265 | 0.278 | 0.265 | 0.199 | 0.418 | 0.258 | 0.272 | 0.258 | 0.194 |
| (0.424097, 0.424097, 0.506847) | 0.660 | 0.153 | 0.020 | 0.153 | 0.015 | 0.656 | 0.151 | 0.021 | 0.151 | 0.015 |

| | **5** | | | | | **6** | | | | |
|---|---|---|---|---|---|---|---|---|---|---|
| k-point coordinates | $5d_{xy}$ | $5d_{yz}$ | $5d_{z^2}$ | $5d_{xz}$ | $5d_{x^2-y^2}$ | $5d_{xy}$ | $5d_{yz}$ | $5d_{z^2}$ | $5d_{xz}$ | $5d_{x^2-y^2}$ |
| (0, 0, 0) | 0.081 | 0.045 | 0.849 | 0.045 | 0.115 | 0.081 | 0.045 | 0.847 | 0.045 | 0.115 |
| (0, 0, 0.506847) | 0.017 | 0.387 | 0.172 | 0.389 | 0.409 | 0.017 | 0.388 | 0.171 | 0.387 | 0.408 |
| (0, 0.424097, 0) | 0.181 | 0.255 | 0.903 | 0.016 | 0.165 | 0.180 | 0.256 | 0.902 | 0.016 | 0.165 |
| (0, 0.424097, 0.506847) | 0.141 | 0.209 | 0.080 | 0.391 | 0.239 | 0.139 | 0.203 | 0.079 | 0.390 | 0.238 |
| (0.424097, 0, 0) | 0.180 | 0.016 | 0.903 | 0.256 | 0.165 | 0.180 | 0.016 | 0.903 | 0.255 | 0.165 |
| (0.424097, 0, 0.506847) | 0.138 | 0.390 | 0.080 | 0.200 | 0.238 | 0.137 | 0.390 | 0.080 | 0.200 | 0.238 |
| (0.424097, 0.424097, 0) | 0.360 | 0.241 | 1.037 | 0.242 | 0.182 | 0.359 | 0.242 | 1.037 | 0.241 | 0.182 |
| (0.424097, 0.424097, 0.506847) | 0.599 | 0.146 | 0.026 | 0.147 | 0.016 | 0.597 | 0.147 | 0.026 | 0.146 | 0.016 |

| | **7** | | | | | **10** | | | | |
|---|---|---|---|---|---|---|---|---|---|---|
| k-point coordinates | $5d_{xy}$ | $5d_{yz}$ | $5d_{z^2}$ | $5d_{xz}$ | $5d_{x^2-y^2}$ | $5d_{xy}$ | $5d_{yz}$ | $5d_{z^2}$ | $5d_{xz}$ | $5d_{x^2-y^2}$ |
| (0, 0, 0) | 0.074 | 0.043 | 0.840 | 0.043 | 0.114 | 0.117 | 0.060 | 0.952 | 0.060 | 0.116 |
| (0, 0, 0.506847) | 0.018 | 0.382 | 0.169 | 0.382 | 0.400 | 0.017 | 0.413 | 0.166 | 0.413 | 0.426 |
| (0, 0.424097, 0) | 0.178 | 0.252 | 0.905 | 0.016 | 0.161 | 0.192 | 0.272 | 0.180 | 0.017 | 0.150 |
| (0, 0.424097, 0.506847) | 0.132 | 0.198 | 0.078 | 0.385 | 0.233 | 0.204 | 0.234 | 0.077 | 0.415 | 0.253 |
| (0.424097, 0, 0) | 0.178 | 0.016 | 0.905 | 0.252 | 0.161 | 0.192 | 0.017 | 0.180 | 0.272 | 0.150 |
| (0.424097, 0, 0.506847) | 0.132 | 0.385 | 0.078 | 0.198 | 0.233 | 0.204 | 0.415 | 0.077 | 0.234 | 0.253 |
| (0.424097, 0.424097, 0) | 0.352 | 0.238 | 1.032 | 0.238 | 0.177 | 0.420 | 0.258 | 0.271 | 0.258 | 0.194 |
| (0.424097, 0.424097, 0.506847) | 1.192 | 0.145 | 0.026 | 0.145 | 0.016 | 0.628 | 0.151 | 0.021 | 0.151 | 0.016 |

| | **11** | | | | | **12** | | | | |
|---|---|---|---|---|---|---|---|---|---|---|
| k-point coordinates | $5d_{xy}$ | $5d_{yz}$ | $5d_{z^2}$ | $5d_{xz}$ | $5d_{x^2-y^2}$ | $5d_{xy}$ | $5d_{yz}$ | $5d_{z^2}$ | $5d_{xz}$ | $5d_{x^2-y^2}$ |
| (0, 0, 0) | 0.092 | 0.050 | 0.873 | 0.050 | 0.115 | 0.096 | 0.051 | 0.874 | 0.051 | 0.131 |
| (0, 0, 0.506847) | 0.017 | 0.396 | 0.169 | 0.396 | 0.414 | 0.017 | 0.396 | 0.169 | 0.396 | 0.414 |
| (0, 0.424097, 0) | 0.184 | 0.261 | 0.888 | 0.017 | 0.173 | 0.184 | 0.261 | 0.889 | 0.017 | 0.173 |
| (0, 0.424097, 0.506847) | 0.161 | 0.205 | 0.078 | 0.399 | 0.243 | 0.167 | 0.207 | 0.079 | 0.399 | 0.243 |
| (0.424097, 0, 0) | 0.184 | 0.017 | 0.888 | 0.261 | 0.173 | 0.184 | 0.017 | 0.889 | 0.261 | 0.173 |
| (0.424097, 0, 0.506847) | 0.161 | 0.399 | 0.078 | 0.205 | 0.243 | 0.167 | 0.399 | 0.079 | 0.207 | 0.243 |
| (0.424097, 0.424097, 0) | 0.382 | 0.247 | 0.255 | 0.247 | 0.185 | 0.383 | 0.247 | 0.258 | 0.247 | 0.185 |
| (0.424097, 0.424097, 0.506847) | 0.610 | 0.148 | 0.024 | 0.148 | 0.016 | 0.610 | 0.148 | 0.024 | 0.148 | 0.016 |

TABLE S9: Lowdin k-resolved spin-summed orbital populations on Nd of the scGW **Solutions 13–20**.

| | **13** | | | | | **14** | | | | |
|---|---|---|---|---|---|---|---|---|---|---|
| k-point coordinates | $5d_{xy}$ | $5d_{yz}$ | $5d_{z^2}$ | $5d_{xz}$ | $5d_{x^2-y^2}$ | $5d_{xy}$ | $5d_{yz}$ | $5d_{z^2}$ | $5d_{xz}$ | $5d_{x^2-y^2}$ |
| (0, 0, 0) | 0.075 | 0.044 | 1.481 | 0.044 | 0.114 | 0.085 | 0.047 | 0.857 | 0.047 | 0.132 |
| (0, 0, 0.506847) | 0.018 | 0.385 | 0.170 | 0.385 | 0.401 | 0.018 | 0.392 | 0.167 | 0.392 | 0.407 |
| (0, 0.424097, 0) | 0.178 | 0.254 | 0.884 | 0.017 | 0.175 | 0.182 | 0.258 | 0.890 | 0.017 | 0.170 |
| (0, 0.424097, 0.506847) | 0.136 | 0.200 | 0.078 | 0.388 | 0.234 | 0.153 | 0.204 | 0.077 | 0.394 | 0.238 |
| (0.424097, 0, 0) | 0.178 | 0.017 | 0.884 | 0.254 | 0.175 | 0.182 | 0.017 | 0.890 | 0.258 | 0.170 |
| (0.424097, 0, 0.506847) | 0.136 | 0.388 | 0.078 | 0.199 | 0.234 | 0.153 | 0.394 | 0.077 | 0.204 | 0.238 |
| (0.424097, 0.424097, 0) | 0.354 | 0.240 | 0.241 | 0.240 | 0.177 | 0.373 | 0.244 | 0.247 | 0.244 | 0.181 |
| (0.424097, 0.424097, 0.506847) | 1.200 | 0.146 | 0.025 | 0.146 | 0.016 | 1.214 | 0.147 | 0.024 | 0.147 | 0.016 |

| | **15** | | | | | **16** | | | | |
|---|---|---|---|---|---|---|---|---|---|---|
| k-point coordinates | $5d_{xy}$ | $5d_{yz}$ | $5d_{z^2}$ | $5d_{xz}$ | $5d_{x^2-y^2}$ | $5d_{xy}$ | $5d_{yz}$ | $5d_{z^2}$ | $5d_{xz}$ | $5d_{x^2-y^2}$ |
| (0, 0, 0) | 0.086 | 0.047 | 1.462 | 0.046 | 0.116 | 0.075 | 0.042 | 1.441 | 0.044 | 0.115 |
| (0, 0, 0.506847) | 0.018 | 0.395 | 0.169 | 0.395 | 0.409 | 0.018 | 0.387 | 0.173 | 0.389 | 0.405 |
| (0, 0.424097, 0) | 0.184 | 0.260 | 0.181 | 0.017 | 0.145 | 0.180 | 0.256 | 0.883 | 0.017 | 0.176 |
| (0, 0.424097, 0.506847) | 0.146 | 0.204 | 0.076 | 0.398 | 0.239 | 0.122 | 0.201 | 0.078 | 0.393 | 0.236 |
| (0.424097, 0, 0) | 0.184 | 0.017 | 0.876 | 0.260 | 0.183 | 0.180 | 0.017 | 0.879 | 0.257 | 0.178 |
| (0.424097, 0, 0.506847) | 0.152 | 0.398 | 0.077 | 0.207 | 0.239 | 0.129 | 0.390 | 0.079 | 0.204 | 0.229 |
| (0.424097, 0.424097, 0) | 0.372 | 0.246 | 0.248 | 0.246 | 0.183 | 0.349 | 0.241 | 0.242 | 0.243 | 0.179 |
| (0.424097, 0.424097, 0.506847) | 1.211 | 0.148 | 0.023 | 0.148 | 0.016 | 1.190 | 0.146 | 0.024 | 0.147 | 0.016 |

| | **17** | | | | | **18** | | | | |
|---|---|---|---|---|---|---|---|---|---|---|
| k-point coordinates | $5d_{xy}$ | $5d_{yz}$ | $5d_{z^2}$ | $5d_{xz}$ | $5d_{x^2-y^2}$ | $5d_{xy}$ | $5d_{yz}$ | $5d_{z^2}$ | $5d_{xz}$ | $5d_{x^2-y^2}$ |
| (0, 0, 0) | 0.082 | 0.045 | 0.929 | 0.044 | 0.113 | 0.083 | 0.046 | 0.849 | 0.046 | 0.114 |
| (0, 0, 0.506847) | 0.018 | 0.393 | 0.170 | 0.393 | 0.409 | 0.018 | 0.392 | 0.168 | 0.392 | 0.407 |
| (0, 0.424097, 0) | 0.184 | 0.260 | 0.876 | 0.017 | 0.184 | 0.183 | 0.259 | 0.889 | 0.017 | 0.170 |
| (0, 0.424097, 0.506847) | 0.137 | 0.203 | 0.078 | 0.396 | 0.239 | 0.145 | 0.202 | 0.077 | 0.395 | 0.238 |
| (0.424097, 0, 0) | 0.183 | 0.017 | 0.851 | 0.260 | 0.199 | 0.182 | 0.017 | 0.888 | 0.259 | 0.170 |
| (0.424097, 0, 0.506847) | 0.141 | 0.396 | 0.077 | 0.207 | 0.238 | 0.148 | 0.395 | 0.077 | 0.205 | 0.237 |
| (0.424097, 0.424097, 0) | 0.365 | 0.246 | 0.247 | 0.246 | 0.181 | 0.370 | 0.244 | 0.246 | 0.245 | 0.181 |
| (0.424097, 0.424097, 0.506847) | 1.201 | 0.148 | 0.024 | 0.148 | 0.016 | 1.210 | 0.147 | 0.024 | 0.148 | 0.016 |

| | **19** | | | | | **20** | | | | |
|---|---|---|---|---|---|---|---|---|---|---|
| k-point coordinates | $5d_{xy}$ | $5d_{yz}$ | $5d_{z^2}$ | $5d_{xz}$ | $5d_{x^2-y^2}$ | $5d_{xy}$ | $5d_{yz}$ | $5d_{z^2}$ | $5d_{xz}$ | $5d_{x^2-y^2}$ |
| (0, 0, 0) | 0.084 | 0.046 | 0.849 | 0.046 | 0.115 | 0.084 | 0.046 | 0.849 | 0.046 | 0.115 |
| (0, 0, 0.506847) | 0.018 | 0.392 | 0.168 | 0.393 | 0.408 | 0.018 | 0.392 | 0.168 | 0.393 | 0.408 |
| (0, 0.424097, 0) | 0.183 | 0.259 | 0.889 | 0.017 | 0.170 | 0.183 | 0.259 | 0.889 | 0.017 | 0.170 |
| (0, 0.424097, 0.506847) | 0.144 | 0.202 | 0.077 | 0.396 | 0.238 | 0.144 | 0.202 | 0.077 | 0.396 | 0.238 |
| (0.424097, 0, 0) | 0.183 | 0.017 | 0.888 | 0.259 | 0.171 | 0.183 | 0.017 | 0.888 | 0.259 | 0.171 |
| (0.424097, 0, 0.506847) | 0.148 | 0.395 | 0.077 | 0.206 | 0.236 | 0.148 | 0.395 | 0.077 | 0.206 | 0.236 |
| (0.424097, 0.424097, 0) | 0.369 | 0.244 | 0.246 | 0.245 | 0.181 | 0.369 | 0.244 | 0.246 | 0.245 | 0.181 |
| (0.424097, 0.424097, 0.506847) | 1.210 | 0.147 | 0.024 | 0.148 | 0.016 | 1.210 | 0.147 | 0.024 | 0.148 | 0.016 |

TABLE S10: Lowdin k-resolved spin-summed orbital populations on Ni of scGW **Solutions 3–7, 10–12**.

| | **3** | | | | | **4** | | | | |
|---|---|---|---|---|---|---|---|---|---|---|
| k-point coordinates | $5d_{xy}$ | $5d_{yz}$ | $5d_{z^2}$ | $5d_{xz}$ | $5d_{x^2-y^2}$ | $5d_{xy}$ | $5d_{yz}$ | $5d_{z^2}$ | $5d_{xz}$ | $5d_{x^2-y^2}$ |
| (0, 0, 0) | 1.612 | 1.697 | 1.184 | 1.697 | 0.830 | 1.615 | 1.697 | 1.388 | 1.697 | 0.829 |
| (0, 0, 0.506847) | 1.666 | 1.661 | 1.668 | 1.661 | 0.834 | 1.665 | 1.662 | 1.671 | 1.662 | 0.833 |
| (0, 0.424097, 0) | 1.666 | 1.677 | 1.551 | 1.704 | 0.862 | 1.664 | 1.676 | 1.564 | 1.703 | 0.859 |
| (0, 0.424097, 0.506847) | 1.648 | 1.656 | 1.653 | 1.511 | 0.869 | 1.645 | 1.656 | 1.656 | 1.519 | 0.869 |
| (0.424097, 0, 0) | 1.666 | 1.704 | 1.551 | 1.677 | 0.862 | 1.664 | 1.703 | 1.564 | 1.676 | 0.859 |
| (0.424097, 0, 0.506847) | 1.648 | 1.511 | 1.653 | 1.656 | 0.869 | 1.645 | 1.519 | 1.656 | 1.656 | 0.869 |
| (0.424097, 0.424097, 0) | 1.636 | 1.667 | 1.415 | 1.667 | 0.934 | 1.636 | 1.665 | 1.432 | 1.665 | 0.651 |
| (0.424097, 0.424097, 0.506847) | 1.650 | 1.673 | 1.649 | 1.673 | 0.665 | 1.648 | 1.673 | 1.651 | 1.673 | 0.657 |

| | **5** | | | | | **6** | | | | |
|---|---|---|---|---|---|---|---|---|---|---|
| k-point coordinates | $5d_{xy}$ | $5d_{yz}$ | $5d_{z^2}$ | $5d_{xz}$ | $5d_{x^2-y^2}$ | $5d_{xy}$ | $5d_{yz}$ | $5d_{z^2}$ | $5d_{xz}$ | $5d_{x^2-y^2}$ |
| (0, 0, 0) | 1.625 | 1.693 | 1.509 | 1.693 | 0.825 | 1.625 | 1.692 | 1.507 | 1.693 | 0.828 |
| (0, 0, 0.506847) | 1.656 | 1.662 | 1.631 | 1.662 | 0.846 | 1.656 | 1.662 | 1.623 | 1.662 | 0.850 |
| (0, 0.424097, 0) | 1.651 | 1.666 | 1.543 | 1.694 | 0.380 | 1.651 | 1.665 | 1.538 | 1.694 | 0.391 |
| (0, 0.424097, 0.506847) | 1.632 | 1.655 | 1.627 | 1.559 | 0.908 | 1.632 | 1.654 | 1.591 | 1.560 | 0.430 |
| (0.424097, 0, 0) | 1.651 | 1.694 | 1.550 | 1.666 | 0.401 | 1.651 | 1.693 | 1.557 | 1.665 | 0.870 |
| (0.424097, 0, 0.506847) | 1.632 | 1.560 | 1.555 | 1.655 | 0.477 | 1.632 | 1.561 | 1.526 | 1.655 | 0.490 |
| (0.424097, 0.424097, 0) | 1.634 | 1.655 | 1.476 | 1.655 | 0.657 | 1.634 | 1.654 | 1.473 | 1.655 | 0.662 |
| (0.424097, 0.424097, 0.506847) | 1.634 | 1.666 | 1.615 | 1.666 | 0.670 | 1.634 | 1.666 | 1.609 | 1.666 | 0.668 |

| | **7** | | | | | **10** | | | | |
|---|---|---|---|---|---|---|---|---|---|---|
| k-point coordinates | $5d_{xy}$ | $5d_{yz}$ | $5d_{z^2}$ | $5d_{xz}$ | $5d_{x^2-y^2}$ | $5d_{xy}$ | $5d_{yz}$ | $5d_{z^2}$ | $5d_{xz}$ | $5d_{x^2-y^2}$ |
| (0, 0, 0) | 1.625 | 1.689 | 1.543 | 1.689 | 0.804 | 1.615 | 1.697 | 1.366 | 1.697 | 0.829 |
| (0, 0, 0.506847) | 1.651 | 1.660 | 1.662 | 1.660 | 0.809 | 1.665 | 1.661 | 1.670 | 1.661 | 0.833 |
| (0, 0.424097, 0) | 1.646 | 1.661 | 1.600 | 1.689 | 0.352 | 1.663 | 1.675 | 1.560 | 1.704 | 0.861 |
| (0, 0.424097, 0.506847) | 1.627 | 1.652 | 1.644 | 1.564 | 0.402 | 1.645 | 1.656 | 1.654 | 1.518 | 0.870 |
| (0.424097, 0, 0) | 1.646 | 1.689 | 1.600 | 1.661 | 0.352 | 1.663 | 1.704 | 1.560 | 1.675 | 0.861 |
| (0.424097, 0, 0.506847) | 1.627 | 1.564 | 1.644 | 1.652 | 0.402 | 1.645 | 1.518 | 1.654 | 1.656 | 0.870 |
| (0.424097, 0.424097, 0) | 1.629 | 1.651 | 1.503 | 1.651 | 0.649 | 1.636 | 1.665 | 1.430 | 1.665 | 0.651 |
| (0.424097, 0.424097, 0.506847) | 1.628 | 1.663 | 1.642 | 1.663 | 0.655 | 1.647 | 1.672 | 1.650 | 1.672 | 0.657 |

| | **11** | | | | | **12** | | | | |
|---|---|---|---|---|---|---|---|---|---|---|
| k-point coordinates | $5d_{xy}$ | $5d_{yz}$ | $5d_{z^2}$ | $5d_{xz}$ | $5d_{x^2-y^2}$ | $5d_{xy}$ | $5d_{yz}$ | $5d_{z^2}$ | $5d_{xz}$ | $5d_{x^2-y^2}$ |
| (0, 0, 0) | 1.623 | 1.694 | 1.480 | 1.694 | 0.821 | 1.621 | 1.694 | 1.490 | 1.694 | 1.507 |
| (0, 0, 0.506847) | 1.659 | 1.662 | 1.667 | 1.662 | 0.822 | 1.658 | 1.661 | 1.666 | 1.661 | 1.513 |
| (0, 0.424097, 0) | 1.655 | 1.669 | 1.584 | 1.697 | 0.859 | 1.655 | 1.668 | 1.579 | 1.697 | 0.349 |
| (0, 0.424097, 0.506847) | 1.637 | 1.655 | 1.630 | 1.546 | 0.439 | 1.636 | 1.654 | 1.649 | 1.542 | 0.395 |
| (0.424097, 0, 0) | 1.655 | 1.697 | 1.584 | 1.669 | 0.859 | 1.655 | 1.697 | 1.579 | 1.668 | 0.349 |
| (0.424097, 0, 0.506847) | 1.637 | 1.546 | 1.630 | 1.655 | 0.439 | 1.636 | 1.542 | 1.649 | 1.654 | 0.395 |
| (0.424097, 0.424097, 0) | 1.633 | 1.659 | 1.471 | 1.659 | 0.652 | 1.631 | 1.658 | 1.468 | 1.658 | 0.631 |
| (0.424097, 0.424097, 0.506847) | 1.638 | 1.668 | 1.646 | 1.668 | 0.652 | 1.638 | 1.667 | 1.646 | 1.667 | 0.637 |

TABLE S11: Lowdin k-resolved spin-summed orbital populations on Ni of scGW **Solutions 13–20**.

| | **13** | | | | | **14** | | | | |
|---|---|---|---|---|---|---|---|---|---|---|
| k-point coordinates | $5d_{xy}$ | $5d_{yz}$ | $5d_{z^2}$ | $5d_{xz}$ | $5d_{x^2-y^2}$ | $5d_{xy}$ | $5d_{yz}$ | $5d_{z^2}$ | $5d_{xz}$ | $5d_{x^2-y^2}$ |
| (0, 0, 0) | 1.624 | 1.690 | 1.644 | 1.690 | 0.804 | 1.623 | 1.691 | 1.511 | 1.691 | 1.495 |
| (0, 0, 0.506847) | 1.652 | 1.660 | 1.664 | 1.660 | 0.808 | 1.655 | 1.660 | 1.663 | 1.660 | 0.819 |
| (0, 0.424097, 0) | 1.646 | 1.662 | 1.602 | 1.690 | 0.345 | 1.650 | 1.664 | 1.589 | 1.692 | 0.348 |
| (0, 0.424097, 0.506847) | 1.627 | 1.652 | 1.646 | 1.563 | 0.395 | 1.631 | 1.652 | 1.646 | 1.552 | 0.392 |
| (0.424097, 0, 0) | 1.646 | 1.690 | 1.602 | 1.662 | 0.345 | 1.650 | 1.692 | 1.589 | 1.664 | 0.348 |
| (0.424097, 0, 0.506847) | 1.627 | 1.563 | 1.646 | 1.652 | 0.395 | 1.631 | 1.552 | 1.646 | 1.652 | 0.392 |
| (0.424097, 0.424097, 0) | 1.627 | 1.651 | 1.504 | 1.651 | 0.639 | 1.629 | 1.653 | 1.484 | 1.653 | 0.637 |
| (0.424097, 0.424097, 0.506847) | 1.629 | 1.663 | 1.643 | 1.663 | 0.646 | 1.633 | 1.664 | 1.643 | 1.664 | 0.641 |

| | **15** | | | | | **16** | | | | |
|---|---|---|---|---|---|---|---|---|---|---|
| k-point coordinates | $5d_{xy}$ | $5d_{yz}$ | $5d_{z^2}$ | $5d_{xz}$ | $5d_{x^2-y^2}$ | $5d_{xy}$ | $5d_{yz}$ | $5d_{z^2}$ | $5d_{xz}$ | $5d_{x^2-y^2}$ |
| (0, 0, 0) | 1.624 | 1.692 | 1.545 | 1.691 | 0.906 | 1.625 | 1.689 | 1.630 | 1.579 | 0.921 |
| (0, 0, 0.506847) | 1.656 | 1.661 | 1.572 | 1.661 | 0.894 | 1.653 | 1.660 | 1.642 | 1.378 | 0.396 |
| (0, 0.424097, 0) | 1.652 | 1.666 | 1.519 | 1.692 | 0.885 | 1.648 | 1.661 | 1.611 | 1.597 | 0.927 |
| (0, 0.424097, 0.506847) | 1.633 | 1.654 | 1.438 | 1.557 | 0.532 | 1.629 | 1.652 | 1.634 | 1.406 | 0.503 |
| (0.424097, 0, 0) | 1.652 | 1.694 | 1.477 | 1.664 | 0.422 | 1.647 | 1.689 | 1.592 | 1.400 | 0.546 |
| (0.424097, 0, 0.506847) | 1.633 | 1.553 | 1.489 | 1.653 | 0.474 | 1.629 | 1.567 | 1.636 | 1.421 | 0.540 |
| (0.424097, 0.424097, 0) | 1.631 | 1.655 | 1.442 | 1.654 | 0.662 | 1.628 | 1.650 | 1.509 | 1.530 | 0.699 |
| (0.424097, 0.424097, 0.506847) | 1.635 | 1.666 | 1.563 | 1.665 | 0.673 | 1.630 | 1.663 | 1.635 | 1.546 | 0.700 |

| | **17** | | | | | **18** | | | | |
|---|---|---|---|---|---|---|---|---|---|---|
| k-point coordinates | $5d_{xy}$ | $5d_{yz}$ | $5d_{z^2}$ | $5d_{xz}$ | $5d_{x^2-y^2}$ | $5d_{xy}$ | $5d_{yz}$ | $5d_{z^2}$ | $5d_{xz}$ | $5d_{x^2-y^2}$ |
| (0, 0, 0) | 1.625 | 1.690 | 1.361 | 1.690 | 0.837 | 1.624 | 1.691 | 1.489 | 1.691 | 0.832 |
| (0, 0, 0.506847) | 1.655 | 1.660 | 1.547 | 1.660 | 0.910 | 1.655 | 1.661 | 1.609 | 1.661 | 0.859 |
| (0, 0.424097, 0) | 1.651 | 1.663 | 1.500 | 1.690 | 0.892 | 1.651 | 1.664 | 1.545 | 1.692 | 0.872 |
| (0, 0.424097, 0.506847) | 1.632 | 1.653 | 1.379 | 1.562 | 0.569 | 1.632 | 1.653 | 1.497 | 1.557 | 0.503 |
| (0.424097, 0, 0) | 1.651 | 1.691 | 1.424 | 1.662 | 0.459 | 1.651 | 1.692 | 1.522 | 1.664 | 0.396 |
| (0.424097, 0, 0.506847) | 1.632 | 1.559 | 1.408 | 1.652 | 0.520 | 1.632 | 1.555 | 1.565 | 1.653 | 0.437 |
| (0.424097, 0.424097, 0) | 1.630 | 1.653 | 1.426 | 1.652 | 0.680 | 1.630 | 1.654 | 1.461 | 1.653 | 0.658 |
| (0.424097, 0.424097, 0.506847) | 1.633 | 1.664 | 1.527 | 1.663 | 0.694 | 1.633 | 1.665 | 1.597 | 1.664 | 0.666 |

| | **19** | | | | | **20** | | | | |
|---|---|---|---|---|---|---|---|---|---|---|
| k-point coordinates | $5d_{xy}$ | $5d_{yz}$ | $5d_{z^2}$ | $5d_{xz}$ | $5d_{x^2-y^2}$ | $5d_{xy}$ | $5d_{yz}$ | $5d_{z^2}$ | $5d_{xz}$ | $5d_{x^2-y^2}$ |
| (0, 0, 0) | 1.624 | 1.691 | 1.503 | 1.665 | 0.842 | 1.624 | 1.691 | 1.503 | 1.664 | 0.842 |
| (0, 0, 0.506847) | 1.655 | 1.661 | 1.638 | 1.637 | 0.855 | 1.655 | 1.661 | 1.638 | 1.637 | 0.855 |
| (0, 0.424097, 0) | 1.651 | 1.664 | 1.566 | 1.671 | 0.877 | 1.651 | 1.664 | 1.566 | 1.671 | 0.877 |
| (0, 0.424097, 0.506847) | 1.632 | 1.653 | 1.546 | 1.524 | 0.497 | 1.632 | 1.653 | 1.546 | 1.524 | 0.497 |
| (0.424097, 0, 0) | 1.651 | 1.693 | 1.555 | 1.584 | 0.436 | 1.651 | 1.693 | 1.555 | 1.584 | 0.437 |
| (0.424097, 0, 0.506847) | 1.632 | 1.555 | 1.612 | 1.585 | 0.458 | 1.632 | 1.555 | 1.612 | 1.585 | 0.458 |
| (0.424097, 0.424097, 0) | 1.630 | 1.654 | 1.474 | 1.626 | 0.665 | 1.630 | 1.654 | 1.474 | 1.626 | 0.665 |
| (0.424097, 0.424097, 0.506847) | 1.634 | 1.665 | 1.618 | 1.638 | 0.670 | 1.634 | 1.665 | 1.618 | 1.638 | 0.670 |

TABLE S12: k-point occupations of scGW solutions.

| k-point coordinates | **3** | | **4** | | **5** | | **6** | | **7** | | **10** | |
|---|---|---|---|---|---|---|---|---|---|---|---|---|
| | $n_{k\alpha}$ | $n_{k\beta}$ | $n_{k\alpha}$ | $n_{k\beta}$ | $n_{k\alpha}$ | $n_{k\beta}$ | $n_{k\alpha}$ | $n_{k\beta}$ | $n_{k\alpha}$ | $n_{k\beta}$ | $n_{k\alpha}$ | $n_{k\beta}$ |
| (0, 0, 0) | 24.00 | 20.02 | 24.93 | 20.01 | 23.01 | 21.90 | 23.01 | 21.91 | 23.01 | 21.89 | 23.02 | 21.93 |
| (0, 0, 0.506847) | 24.00 | 20.01 | 24.00 | 20.01 | 23.01 | 20.96 | 23.01 | 20.96 | 23.02 | 20.94 | 23.01 | 21.00 |
| (0, 0.424097, 0) | 23.99 | 20.00 | 23.99 | 20.00 | 23.00 | 21.04 | 23.00 | 21.04 | 23.01 | 21.02 | 23.00 | 20.99 |
| (0, 0.424097, 0.506847) | 23.99 | 20.00 | 23.99 | 20.00 | 23.00 | 20.96 | 23.00 | 20.08 | 23.01 | 20.07 | 23.00 | 20.99 |
| (0.424097, 0, 0) | 23.99 | 20.00 | 23.99 | 20.00 | 23.00 | 21.03 | 23.00 | 21.92 | 23.01 | 21.02 | 23.00 | 20.99 |
| (0.424097, 0, 0.506847) | 23.99 | 20.00 | 23.99 | 20.00 | 23.00 | 20.08 | 23.00 | 20.08 | 23.01 | 20.07 | 23.00 | 20.99 |
| (0.424097, 0.424097, 0) | 23.99 | 20.00 | 23.09 | 20.00 | 23.00 | 21.01 | 23.00 | 21.02 | 23.00 | 21.00 | 23.00 | 20.09 |
| (0.424097, 0.424097, 0.506847) | 24.03 | 19.98 | 24.02 | 19.98 | 22.98 | 21.01 | 22.98 | 21.00 | 23.94 | 20.99 | 22.98 | 21.02 |

| k-point coordinates | **11** | | **12** | | **13** | | **14** | | **15** | | **16** | |
|---|---|---|---|---|---|---|---|---|---|---|---|---|
| | $n_{k\alpha}$ | $n_{k\beta}$ | $n_{k\alpha}$ | $n_{k\beta}$ | $n_{k\alpha}$ | $n_{k\beta}$ | $n_{k\alpha}$ | $n_{k\beta}$ | $n_{k\alpha}$ | $n_{k\beta}$ | $n_{k\alpha}$ | $n_{k\beta}$ |
| (0, 0, 0) | 23.01 | 21.92 | 23.90 | 21.87 | 23.95 | 21.88 | 23.88 | 21.87 | 23.95 | 21.89 | 23.95 | 21.88 |
| (0, 0, 0.506847) | 23.01 | 20.97 | 23.90 | 20.92 | 23.02 | 20.94 | 23.04 | 20.93 | 23.02 | 20.94 | 23.02 | 20.08 |
| (0, 0.424097, 0) | 23.00 | 21.92 | 23.04 | 21.02 | 23.02 | 21.01 | 23.03 | 21.02 | 23.02 | 20.96 | 23.02 | 21.88 |
| (0, 0.424097, 0.506847) | 23.00 | 20.09 | 23.04 | 20.07 | 23.02 | 20.06 | 23.03 | 20.06 | 23.02 | 20.07 | 23.02 | 20.06 |
| (0.424097, 0, 0) | 23.00 | 21.92 | 23.04 | 21.02 | 23.02 | 21.01 | 23.03 | 21.02 | 23.02 | 21.02 | 23.02 | 21.01 |
| (0.424097, 0, 0.506847) | 23.00 | 20.09 | 23.04 | 20.07 | 23.02 | 20.06 | 23.03 | 20.06 | 23.01 | 20.07 | 23.02 | 20.06 |
| (0.424097, 0.424097, 0) | 23.00 | 20.09 | 23.03 | 20.06 | 23.01 | 20.06 | 23.02 | 20.06 | 23.02 | 20.06 | 23.01 | 20.06 |
| (0.424097, 0.424097, 0.506847) | 22.98 | 21.01 | 23.01 | 20.98 | 23.95 | 20.98 | 23.95 | 20.98 | 23.95 | 20.99 | 23.95 | 20.98 |

| k-point coordinates | **17** | | **18** | | **19** | | **20** | | | | | |
|---|---|---|---|---|---|---|---|---|---|---|---|---|
| | $n_{k\alpha}$ | $n_{k\beta}$ | $n_{k\alpha}$ | $n_{k\beta}$ | $n_{k\alpha}$ | $n_{k\beta}$ | $n_{k\alpha}$ | $n_{k\beta}$ | $n_{k\alpha}$ | $n_{k\beta}$ | $n_{k\alpha}$ | $n_{k\beta}$ |
| (0, 0, 0) | 23.96 | 20.96 | 23.01 | 21.90 | 23.01 | 21.90 | 23.01 | 21.90 | | | | |
| (0, 0, 0.506847) | 23.03 | 20.93 | 23.01 | 20.95 | 23.01 | 20.95 | 23.01 | 20.95 | | | | |
| (0, 0.424097, 0) | 23.97 | 20.94 | 23.01 | 21.90 | 23.01 | 21.90 | 23.01 | 21.90 | | | | |
| (0, 0.424097, 0.506847) | 23.02 | 20.06 | 23.01 | 20.07 | 23.01 | 20.07 | 23.01 | 20.07 | | | | |
| (0.424097, 0, 0) | 23.02 | 21.00 | 23.00 | 21.03 | 23.00 | 21.03 | 23.00 | 21.03 | | | | |
| (0.424097, 0, 0.506847) | 23.02 | 20.06 | 23.01 | 20.08 | 23.01 | 20.08 | 23.01 | 20.08 | | | | |
| (0.424097, 0.424097, 0) | 23.03 | 20.05 | 23.01 | 20.07 | 23.01 | 20.07 | 23.01 | 20.07 | | | | |
| (0.424097, 0.424097, 0.506847) | 23.95 | 20.98 | 23.94 | 20.99 | 23.94 | 20.99 | 23.94 | 20.99 | | | | |

TABLE S13: Sigmas between UHF solutions

| | 1 | 2 | 3 | 4 | 5 | 6 | 7 | 8 | 9 | 10 | 11 | 13 | 14 | 15 | 16 | 17 | 18 | 19 | 20 |
|---|---|---|---|---|---|---|---|---|---|---|---|---|---|---|---|---|---|---|---|
| 1 | 0 | 1.00 | 1.00 | 1.00 | 1.00 | 1.00 | 1.00 | 1.00 | 1.00 | 1.00 | 1.00 | 1.00 | 1.00 | 1.00 | 1.00 | 1.00 | 1.00 | 1.00 | 1.00 |
| 2 | 1.00 | 0 | 1.00 | 1.00 | 1.00 | 1.00 | 1.00 | 1.00 | 1.00 | 1.00 | 1.00 | 1.00 | 1.00 | 1.00 | 1.00 | 1.00 | 1.00 | 1.00 | 1.00 |
| 3 | 1.00 | 1.00 | 0 | 1.00 | 1.00 | 1.00 | 1.00 | 1.00 | 1.00 | 1.00 | 1.00 | 1.00 | 1.00 | 1.00 | 1.00 | 1.00 | 1.00 | 1.00 | 1.00 |
| 4 | 1.00 | 1.00 | 1.00 | 0 | 1.00 | 1.00 | 1.00 | 1.00 | 1.00 | 1.00 | 1.00 | 1.00 | 1.00 | 1.00 | 1.00 | 1.00 | 1.00 | 1.00 | 1.00 |
| 5 | 1.00 | 1.00 | 1.00 | 1.00 | 0 | 1.00 | 1.00 | 1.00 | 0.53 | 1.00 | 1.00 | 1.00 | 1.00 | 1.00 | 1.00 | 1.00 | 1.00 | 1.00 | 1.00 |
| 6 | 1.00 | 1.00 | 1.00 | 1.00 | 1.00 | 0 | 1.00 | 1.00 | 1.00 | 1.00 | 1.00 | 1.00 | 1.00 | 1.00 | 1.00 | 1.00 | 1.00 | 1.00 | 1.00 |
| 7 | 1.00 | 1.00 | 1.00 | 1.00 | 1.00 | 1.00 | 0 | 1.00 | 1.00 | 1.00 | 1.00 | 1.00 | 1.00 | 1.00 | 1.00 | 1.00 | 1.00 | 1.00 | 1.00 |
| 8 | 1.00 | 1.00 | 1.00 | 1.00 | 1.00 | 1.00 | 1.00 | 0 | 1.00 | 1.00 | 1.00 | 1.00 | 1.00 | 1.00 | 1.00 | 1.00 | 1.00 | 1.00 | 1.00 |
| 9 | 1.00 | 1.00 | 1.00 | 1.00 | 0.53 | 1.00 | 1.00 | 1.00 | 0 | 1.00 | 1.00 | 1.00 | 1.00 | 1.00 | 1.00 | 1.00 | 1.00 | 1.00 | 1.00 |
| 10 | 1.00 | 1.00 | 1.00 | 1.00 | 1.00 | 1.00 | 1.00 | 1.00 | 1.00 | 0 | 1.00 | 1.00 | 1.00 | 1.00 | 1.00 | 1.00 | 1.00 | 1.00 | 1.00 |
| 11 | 1.00 | 1.00 | 1.00 | 1.00 | 1.00 | 1.00 | 1.00 | 1.00 | 1.00 | 1.00 | 0 | 1.00 | 1.00 | 1.00 | 1.00 | 1.00 | 1.00 | 1.00 | 1.00 |
| 13 | 1.00 | 1.00 | 1.00 | 1.00 | 1.00 | 1.00 | 1.00 | 1.00 | 1.00 | 1.00 | 1.00 | 0 | 1.00 | 1.00 | 1.00 | 1.00 | 1.00 | 1.00 | 1.00 |
| 14 | 1.00 | 1.00 | 1.00 | 1.00 | 1.00 | 1.00 | 1.00 | 1.00 | 1.00 | 1.00 | 1.00 | 1.00 | 0 | 1.00 | 1.00 | 1.00 | 1.00 | 1.00 | 1.00 |
| 15 | 1.00 | 1.00 | 1.00 | 1.00 | 1.00 | 1.00 | 1.00 | 1.00 | 1.00 | 1.00 | 1.00 | 1.00 | 1.00 | 0 | 1.00 | 1.00 | 1.00 | 1.00 | 1.00 |
| 16 | 1.00 | 1.00 | 1.00 | 1.00 | 1.00 | 1.00 | 1.00 | 1.00 | 1.00 | 1.00 | 1.00 | 1.00 | 1.00 | 1.00 | 0 | 1.00 | 1.00 | 1.00 | 1.00 |
| 17 | 1.00 | 1.00 | 1.00 | 1.00 | 1.00 | 1.00 | 1.00 | 1.00 | 1.00 | 1.00 | 1.00 | 1.00 | 1.00 | 1.00 | 1.00 | 0 | 1.00 | 1.00 | 1.00 |
| 18 | 1.00 | 1.00 | 1.00 | 1.00 | 1.00 | 1.00 | 1.00 | 1.00 | 1.00 | 1.00 | 1.00 | 1.00 | 1.00 | 1.00 | 1.00 | 1.00 | 0 | 0.00 | 0.00 |
| 19 | 1.00 | 1.00 | 1.00 | 1.00 | 1.00 | 1.00 | 1.00 | 1.00 | 1.00 | 1.00 | 1.00 | 1.00 | 1.00 | 1.00 | 1.00 | 1.00 | 0.00 | 0 | 0.00 |
| 20 | 1.00 | 1.00 | 1.00 | 1.00 | 1.00 | 1.00 | 1.00 | 1.00 | 1.00 | 1.00 | 1.00 | 1.00 | 1.00 | 1.00 | 1.00 | 1.00 | 0.00 | 0.00 | 0 |

TABLE S14: Sigmas between scGW solutions

| | 3 | 4 | 5 | 6 | 7 | 10 | 11 | 12 | 13 | 14 | 15 | 16 | 17 | 18 | 19 | 20 |
|---|---|---|---|---|---|---|---|---|---|---|---|---|---|---|---|---|
| 3 | 0 | 0.94 | 0.97 | 0.97 | 0.97 | 0.97 | 0.97 | 0.96 | 0.97 | 0.96 | 0.97 | 0.97 | 0.97 | 0.97 | 0.97 | 0.97 |
| 4 | 0.94 | 0 | 0.96 | 0.96 | 0.96 | 0.97 | 0.96 | 0.96 | 0.96 | 0.96 | 0.96 | 0.96 | 0.96 | 0.96 | 0.96 | 0.96 |
| 5 | 0.97 | 0.96 | 0 | 0.89 | 0.96 | 0.96 | 0.94 | 0.94 | 0.96 | 0.96 | 0.96 | 0.96 | 0.96 | 0.96 | 0.96 | 0.96 |
| 6 | 0.97 | 0.96 | 0.89 | 0 | 0.96 | 0.96 | 0.94 | 0.94 | 0.96 | 0.96 | 0.96 | 0.96 | 0.96 | 0.96 | 0.96 | 0.96 |
| 7 | 0.97 | 0.96 | 0.96 | 0.96 | 0 | 0.96 | 0.96 | 0.96 | 0.94 | 0.94 | 0.95 | 0.94 | 0.96 | 0.94 | 0.94 | 0.94 |
| 10 | 0.97 | 0.97 | 0.96 | 0.96 | 0.96 | 0 | 0.95 | 0.95 | 0.96 | 0.96 | 0.96 | 0.96 | 0.96 | 0.96 | 0.96 | 0.96 |
| 11 | 0.97 | 0.96 | 0.94 | 0.94 | 0.96 | 0.95 | 0 | 0.89 | 0.96 | 0.96 | 0.96 | 0.96 | 0.96 | 0.96 | 0.96 | 0.96 |
| 12 | 0.96 | 0.96 | 0.94 | 0.94 | 0.96 | 0.95 | 0.89 | 0 | 0.96 | 0.96 | 0.96 | 0.96 | 0.96 | 0.96 | 0.96 | 0.96 |
| 13 | 0.97 | 0.96 | 0.96 | 0.96 | 0.94 | 0.96 | 0.96 | 0.96 | 0 | 0.94 | 0.95 | 0.88 | 0.95 | 0.94 | 0.94 | 0.94 |
| 14 | 0.96 | 0.96 | 0.96 | 0.96 | 0.94 | 0.96 | 0.96 | 0.96 | 0.94 | 0 | 0.95 | 0.92 | 0.95 | 0.89 | 0.89 | 0.89 |
| 15 | 0.97 | 0.96 | 0.96 | 0.96 | 0.95 | 0.96 | 0.96 | 0.96 | 0.95 | 0.95 | 0 | 0.95 | 0.95 | 0.95 | 0.95 | 0.95 |
| 16 | 0.97 | 0.96 | 0.96 | 0.96 | 0.94 | 0.96 | 0.96 | 0.96 | 0.88 | 0.92 | 0.95 | 0 | 0.95 | 0.94 | 0.94 | 0.94 |
| 17 | 0.97 | 0.96 | 0.96 | 0.96 | 0.96 | 0.96 | 0.96 | 0.96 | 0.95 | 0.95 | 0.95 | 0.95 | 0 | 0.95 | 0.95 | 0.95 |
| 18 | 0.97 | 0.96 | 0.96 | 0.96 | 0.94 | 0.96 | 0.96 | 0.96 | 0.94 | 0.89 | 0.95 | 0.94 | 0.95 | 0 | 0.28 | 0.28 |
| 19 | 0.97 | 0.96 | 0.96 | 0.96 | 0.94 | 0.96 | 0.96 | 0.96 | 0.94 | 0.89 | 0.95 | 0.94 | 0.95 | 0.28 | 0 | 0.52 |
| 20 | 0.97 | 0.96 | 0.96 | 0.96 | 0.94 | 0.96 | 0.96 | 0.96 | 0.94 | 0.89 | 0.95 | 0.94 | 0.95 | 0.28 | 0.52 | 0 |

TABLE S15: Sigmas between UHF and scGW solutions

| UHF/scGW | 3 | 4 | 5 | 6 | 7 | 10 | 11 | 12 | 13 | 14 | 15 | 16 | 17 | 18 | 19 | 20 |
|---|---|---|---|---|---|---|---|---|---|---|---|---|---|---|---|---|
| 1 | 0.99 | 0.99 | 0.98 | 0.98 | 0.99 | 0.98 | 0.98 | 0.98 | 0.99 | 0.98 | 0.98 | 0.99 | 0.99 | 0.98 | 0.98 | 0.98 |
| 2 | 0.99 | 0.99 | 0.98 | 0.98 | 0.99 | 0.98 | 0.98 | 0.98 | 0.99 | 0.98 | 0.98 | 0.99 | 0.98 | 0.98 | 0.98 | 0.98 |
| 3 | **0.20** | 0.97 | 0.99 | 0.99 | 0.98 | 0.99 | 0.99 | 0.99 | 0.98 | 0.97 | 0.98 | 0.98 | 0.98 | 0.98 | 0.98 | 0.98 |
| 4 | 0.97 | **0.19** | 0.99 | 0.99 | 0.98 | 0.99 | 0.99 | 0.99 | 0.98 | 0.98 | 0.98 | 0.98 | 0.98 | 0.98 | 0.98 | 0.98 |
| 5 | 0.99 | 0.99 | **0.31** | 0.95 | 0.97 | 0.98 | 0.97 | 0.97 | 0.97 | 0.97 | 0.98 | 0.97 | 0.98 | 0.97 | 0.97 | 0.97 |
| 6 | 0.99 | 0.99 | 0.95 | **0.50** | 0.97 | 0.98 | 0.97 | 0.97 | 0.97 | 0.97 | 0.98 | 0.97 | 0.98 | 0.97 | 0.97 | 0.97 |
| 7 | 0.99 | 0.99 | 0.99 | 0.99 | **0.15** | 0.99 | 0.99 | 0.99 | 0.97 | 0.97 | 0.97 | 0.97 | 0.98 | 0.97 | 0.97 | 0.97 |
| 8 | 0.99 | 0.99 | 0.98 | 0.98 | 0.99 | 0.98 | 0.98 | 0.98 | 0.99 | 0.98 | 0.98 | 0.99 | 0.98 | 0.98 | 0.98 | 0.98 |
| 9 | 0.99 | 0.99 | 0.35 | 0.95 | 0.97 | 0.98 | 0.97 | 0.97 | 0.97 | 0.97 | 0.98 | 0.97 | 0.98 | 0.97 | 0.97 | 0.97 |
| 10 | 0.99 | 0.99 | 0.97 | 0.97 | 0.97 | **0.21** | 0.97 | 0.97 | 0.97 | 0.97 | 0.97 | 0.97 | 0.97 | 0.97 | 0.97 | 0.97 |
| 11 | 0.99 | 0.99 | 0.97 | 0.97 | 0.97 | 0.98 | **0.18** | 0.94 | 0.97 | 0.97 | 0.98 | 0.97 | 0.99 | 0.97 | 0.97 | 0.97 |
| 13 | 0.99 | 0.99 | 0.99 | 0.99 | 0.98 | 0.99 | 0.99 | 0.99 | **0.15** | 0.98 | 0.98 | 0.94 | 0.99 | 0.98 | 0.98 | 0.98 |
| 14 | 0.99 | 0.99 | 0.99 | 0.99 | 0.99 | 0.99 | 0.99 | 0.99 | 0.99 | **0.96** | 0.99 | 0.99 | 0.99 | 0.99 | 0.99 | 0.99 |
| 15 | 0.99 | 0.99 | 0.99 | 0.99 | 0.98 | 0.99 | 0.99 | 0.99 | 0.97 | 0.97 | **0.46** | 0.97 | 0.97 | 0.98 | 0.98 | 0.98 |
| 16 | 0.99 | 0.99 | 0.99 | 0.99 | 0.98 | 0.99 | 0.99 | 0.99 | 0.95 | 0.96 | 0.98 | **0.34** | 0.99 | 0.98 | 0.98 | 0.98 |
| 17 | 0.99 | 0.99 | 0.99 | 0.99 | 0.99 | 0.99 | 0.99 | 0.99 | 0.98 | 0.99 | 0.98 | 0.98 | **0.50** | 0.99 | 0.99 | 0.99 |
| 18 | 0.99 | 0.99 | 0.99 | 0.99 | 0.97 | 0.99 | 0.99 | 0.99 | 0.96 | 0.95 | 0.98 | 0.96 | 0.98 | **0.47** | 0.58 | 0.58 |
| 19 | 0.99 | 0.99 | 0.99 | 0.99 | 0.97 | 0.99 | 0.99 | 0.99 | 0.96 | 0.95 | 0.98 | 0.96 | 0.98 | 0.47 | **0.58** | 0.58 |
| 20 | 0.99 | 0.99 | 0.99 | 0.99 | 0.97 | 0.99 | 0.99 | 0.99 | 0.96 | 0.95 | 0.98 | 0.96 | 0.98 | 0.47 | 0.58 | **0.58** |
